# Supplementary material for: PanelNet: Understanding 360 Indoor Environment via Panel Representation
Source: arXiv:2305.09078 source file (2023-05-16)
Supplement: Supplementary file 1 [file _supplementary.tex]

\input{_constants}
\cameraready % \review OR \cameraready

\documentclass[10pt,twocolumn,letterpaper]{article}
\input{cvpr_header}
\myexternaldocument{_main}
\begin{document}
%% TITLE
\title{\paperTitle \\ Supplementary Material}
\author{\authorBlock}
\maketitle

\input{12_appendix}

{\small
\bibliographystyle{ieee_fullname}
\bibliography{11_references}
}

\end{document}
